# Supplementary material for: Seg&Struct: The Interplay Between Part Segmentation and Structure Inference for 3D Shape Parsing
Source: arXiv:2211.00382 source file (2022-11-01)
Supplement: Supplementary file 1 [file exp_2.tex]

% https://docs.google.com/spreadsheets/d/1r7HvS48l_Q9RKG1NcRaNjktnm-JdVoTbRei5pe9DQe8/edit?usp=sharing

% \section{Experimental Results}
\section{Training Details}
In this section, we evaluate the performance of our proposed framework for the targeted tasks, including the structure inference, the segmentation refinement, and the shape retrieval as an our application. % retrieval
The main goal of our framework is to build a synergy between part segmentation and the structure prediction.
Therefore, we seek the opportunity for this \emph{interplay} between two different tasks by supporting each other. % in iterative manner.  
This process is represented in both the \emph{forward} and the \emph{backward} path as demonstrated in the previous section.

In the \emph{forward} path, we evaluate the effectiveness of the our segmentation-driven structure prediction, which exploits the association between part regions in the raw 3D shapes and semantic parts in the structure hierarchy (Section~\ref{Sec:6.2}).
In the \emph{backward} path, we verify whether the structure-to-segmentation can refine the noisy part segmentation output utilizing the structure-aware information (Section~\ref{Sec:refinement results}).
To evaluate this, we compare ours to a list of baselines for each task to describe the significance of our method compared to others.
Then, we show our structure inference can be used for a shape retrieval application by qualitatively comparing our \emph{structure-aware} shape retrieval with the chamfer distance-based one. 

\subsection{Data Preparation}
For the experiments, we prepared two kinds of datasets to test our method: PartNet~\cite{mo2019partnet} and StructureNet~\cite{10.1145/3355089.3356527}.
ParNet provides point cloud data sampled on surfaces of 3D mesh from ShapeNet~\cite{chang2015shapenet} and its corresponding semantic-instance part annotation.
We use PartNet to train our parser backbone and evaluate the segmentation refinement experiment.
StructureNet is built upon PartNet with an additional annotation of a structural hierarchy and inter-part relationships. % composed of part instances.
For each parts of a given structure in the dataset, a part geometry is represented as bounding box parameter $\theta$ in global coordinate systems. 
It also contains part-relation such as adjacency and symmetry represented as edge connectivity in one-hot encoded labels between a pair of parts.
Our dataset configuration is analogous to the experiment setup for StructureNet, which has a maximum number of parts in a subset of the tree as 10 and four types of symmetry relations.
We test our method on three largest categories: \textit{chair}, \textit{table}, and \textit{storage furniture}.
Since we evaluate our framework integrating these two dataset, we filter the shapes with invalid annotation such as missing parts annotations.  
The remaining shapes for chair, table, and storage furniture are 3522, 1802, and 932, respectively.
We split these samples into the train and test set following PartNet. % \Jeonghyun{more details?}

% \subsection{Network Training}
% \Jeonghyun{Is it necessary?}

% ------------------------------------------------------------------------------------------------------------------------------------------------------ %
\begin{table*}[]
\centering
\caption{\textbf{Comparison on Structure Inference.} Please note that AP means part prediction accuracy (\%) computed by average precision with IoU threshold 0.25, and EE means edge prediction error calculated by one minus F1-score of edge prediction outputs. The second and third baselines do not measure EE since they do not predict any part relationships. The bold text is used for the best results for each column. The columns for key components describe which prior knowledge or the level of message passing each method takes.}
\begin{tabular}{ll|ccccc|cccccccc}
\hline
\multicolumn{1}{c}{\multirow{3}{*}{Id}} & \multicolumn{1}{c|}{\multirow{3}{*}{Method}}     & \multicolumn{5}{c|}{Key Components}                                                           & \multicolumn{6}{c}{Categories}                                                           & \multicolumn{2}{c}{\multirow{2}{*}{Avg}} \\ \cline{3-13}
\multicolumn{1}{c}{}                    & \multicolumn{1}{c|}{}                            & \multicolumn{2}{c|}{Prior}                       & \multicolumn{3}{c|}{Message Passing}       & \multicolumn{2}{c}{Chair} & \multicolumn{2}{c}{Table} & \multicolumn{2}{c}{Storagefurn.} & \multicolumn{2}{c}{}                     \\ \cline{3-15} 
\multicolumn{1}{c}{}                    & \multicolumn{1}{c|}{}                            & Seg.         & \multicolumn{1}{c|}{Hier.}        & Skip.        & Local        & global       & AP (\%)      & EE (↓)     & AP (\%)      & EE (↓)     & AP (\%)         & EE (↓)         & AP (\%)             & EE (↓)             \\ \hline
1                                       & $\mathcal{F}_s + \mathcal{G}_{SN}$               &              & \multicolumn{1}{c|}{\checkmark} &              & \checkmark & \checkmark & 5.03         & 0.6824     & 2.02         & 0.8272     & 1.07            & 0.6491         & 2.71                & 0.7196             \\ \hline
2                                       & $\psi + \text{PCA}$                              & \checkmark & \multicolumn{1}{c|}{}             &              &              &              & 37.32        & -          & 20.96        & -          & 17.75           & -              & 25.34               & -                  \\
3                                       & $\psi + g_{box}$                                 & \checkmark & \multicolumn{1}{c|}{}             &              &              &              & 46.66        & -          & 25.89        & -          & 19.96           & -              & 30.83               & -                  \\
4                                       & $\psi + g_{box}+g_{mp}$                          & \checkmark & \multicolumn{1}{c|}{}             &              & \checkmark &              & 48.39        & 0.8576     & 24.19        & 0.8835     & 19.96           & 0.8933         & 30.85               & 0.8781             \\ \hline
5                                       & $\mathcal{F} + \mathcal{G}_{SN}$                 & \checkmark & \multicolumn{1}{c|}{\checkmark} &              & \checkmark & \checkmark & 10.79        & 0.4211     & 1.28         & 0.7863     & 1.95            & \textbf{0.5191}         & 4.68                & 0.5755             \\
6                                       & $\mathcal{F} + \mathcal{G} - f_{ctx}$            & \checkmark & \multicolumn{1}{c|}{\checkmark} & \checkmark &              & \checkmark & 47.21        & 0.3006     & 22.91        & 0.4597     & 19.25           & 0.6664         & 29.79               & 0.4756             \\
7                                       & $\mathcal{F} + \mathcal{G} - g_{mp}$             & \checkmark & \multicolumn{1}{c|}{\checkmark} & \checkmark & \checkmark &              & 47.34        & 0.3448     & 26.41        & 0.5024     & 21.2            & 0.6867         & 31.65               & 0.5113             \\
8                                       & $\mathcal{F} + \mathcal{G}$ (Ours)                     & \checkmark & \multicolumn{1}{c|}{\checkmark} & \checkmark & \checkmark & \checkmark & 48.41        & 0.2727     & 26.36        & 0.4400       & 21.57           & 0.6934         & 32.11               & 0.4687             \\ \hline
9                                       & (Ours) $+ \mathcal{M}$ & \checkmark & \multicolumn{1}{c|}{\checkmark} & \checkmark & \checkmark & \checkmark & \textbf{51.41}        & \textbf{0.2581}     & \textbf{27.62}        & \textbf{0.3939}     & \textbf{21.90}           & 0.6928         & \textbf{33.64}              & \textbf{0.4483}             \\ \hline
\end{tabular}
\label{tab:comparison}
\end{table*}

% ------------------------------------------------------------------------------------------------------------------------------------------------------ %

\subsection{Segmentation-driven Structure Inference}\label{Sec:6.2}
In this section, we present the performance of our segmentation-driven structure inference to predict part structure with quantitative and qualitative evaluations.
To show the significance of our proposed method, we compare it to several baselines built upon the naive encoder-decoder architecture. 

We first describe that our method achieves the most accurate and realistic structure exploiting the association between part regions in input shape geometry and semantic parts in the structure.
Then, we discuss about the effectiveness of the other key component, the hierarchical message passing $g_h$, in the ablation studies demonstrating how does it assists our framework to learn co-relations between nodes in the predicted structure.
Through extensive experiments including ablation studies, we find that the segmentation and hierarchy priors promotes structure inference to get both accurate and consistent structure output.

\subsubsection{Baselines}
We compare ours to two encoder-decoder type of baselines, which encode the input into a single feature vector and decode it to predict the whole part structure including part geometry and part-relationships.
First, we build a baseline that consumes the whole raw 3D shape as input, using a shape encoder $\mathcal{F}_s$ and the structure decoder $\mathcal{G}_{SN}$. 
The shape encoder $\mathcal{F}_s$ uses PointNet++ \cite{qi2017pointnetplusplus} architecture adapting four abstraction layers and two feature propagation layers with ReLU activation.
For the structure decoder $\mathcal{G}_{SN}$, we adapt a GNN-based decoder network used in StructureNet~\cite{10.1145/3355089.3356527}, the state-of-the-art method for the structure decoding.
This baseline takes the most naive approach by just aggregating the raw 3D shape into a single latent code without any supervision used in our framework, i.e. part segmentation and hierarchy prior.

Similarly, we build an additional baseline that encodes the extracted part instances into a root feature vector hierarchically using our structure tree encoder $\mathcal{F}$ and decode it using $\mathcal{G}_{SN}$.
While it leverages two types of priors, part segmentation and hierarchy, the second baseline also lacks the most important component in our method: Skip connection.  
By naively adapting the structure decoder $\mathcal{G}_{SN}$, the model still suffers to predict the structure just depending on the single latent code only, while not exploiting any association between between the raw 3D shape and the semantic parts in hierarchy.

Both two baselines cope with the structure prediction in an implicit way, which expects the encoded vector to implicitly contain all the information for the structure.
From them, we aim to tackle drawbacks of the approach without building association between the raw 3D shape and the part structure.
Additionally, we design three more baselines for ablation studies on hierarchical message passing $g_h$ by subtracting key components: local part-relation learning, and global context encoding.
We will discuss it later with more detail in ablation studies. % in Sec~\ref{Sec:6.4}.

\subsubsection{Metrics}
Our goal is to achieve not only accurate but also globally aligned part structure inference.
To this end, our framework predicts oriented bounding box for the part node to abstract the part geometry and part-relations (i.e. symmetry and adjacency) across the nodes in the same subset to make predicted part boxes being co-related to each other.
We evaluate our method using two metrics: part prediction accuracy and edge prediction error.

Part prediction accuracy measures how accurately are part geometry predicted based on decoded bounding boxes compared to the counterpart target part structure.
Since this is conventional objective of the object detection problem~\cite{song2016deep}, we opt to calculate the accuracy using \emph{Average Precision (AP)}.
%Therefore, part prediction accuracy measures the accuracy for each part geometry from bounding box decoder assisted by hierarchical message passing. 
We use a class-agnostic AP since we do not predict any semantics in our structure inference stage, depending on the outputs from the pre-trained part segmentation backbone.
We will discuss about the quality of semantic classification later in refinement evaluation (Section~\ref{refinement results}).
The correspondence between outputs and target structures is established only for the leaf nodes, using similar bipartite matching in the training stage based on bounding box parameters.
We calculate AP with IoU threshold 0.25 for each shape and average the sum by the number of shapes in category. 

Edge prediction error measures whether the relationships between the pair of nodes are predicted well. % On the other hand, 
As mentioned earlier~\ref{4.2}, our part-relationship learning is depending on the edge prediction accuracy. 
This means the lower edge prediction error we have, the more consistent geometry is likely to produced.% \Jeonghyun{True?}
For edge prediction error, we borrow the same metric from StructureNet, using the modified assignment $\hat{\textbf{M}}$ between predicted structure and target structure for the part nodes with the same semantics only. % \Jeonghyun{need to mention the reason?}
We compute the error as one minus F1-score using edge precision $e_p$ and edge recall $e_r$ based on edge prediction outputs: % where $|\cdot|$ means the number of matched nodes: % =\frac{|\hat{\textbf{R}}_{\hat{\textbf{M}}}|}{|\textbf{R}|}, =\frac{|\hat{\textbf{R}}|}{|\textbf{R}|}
\begin{equation}
    EE = 1 - 2 \left( \frac{e_r\times e_p}{e_r+e_p} \right)
\end{equation}

\begin{figure*}
    \centering
    \includegraphics[width=\textwidth]{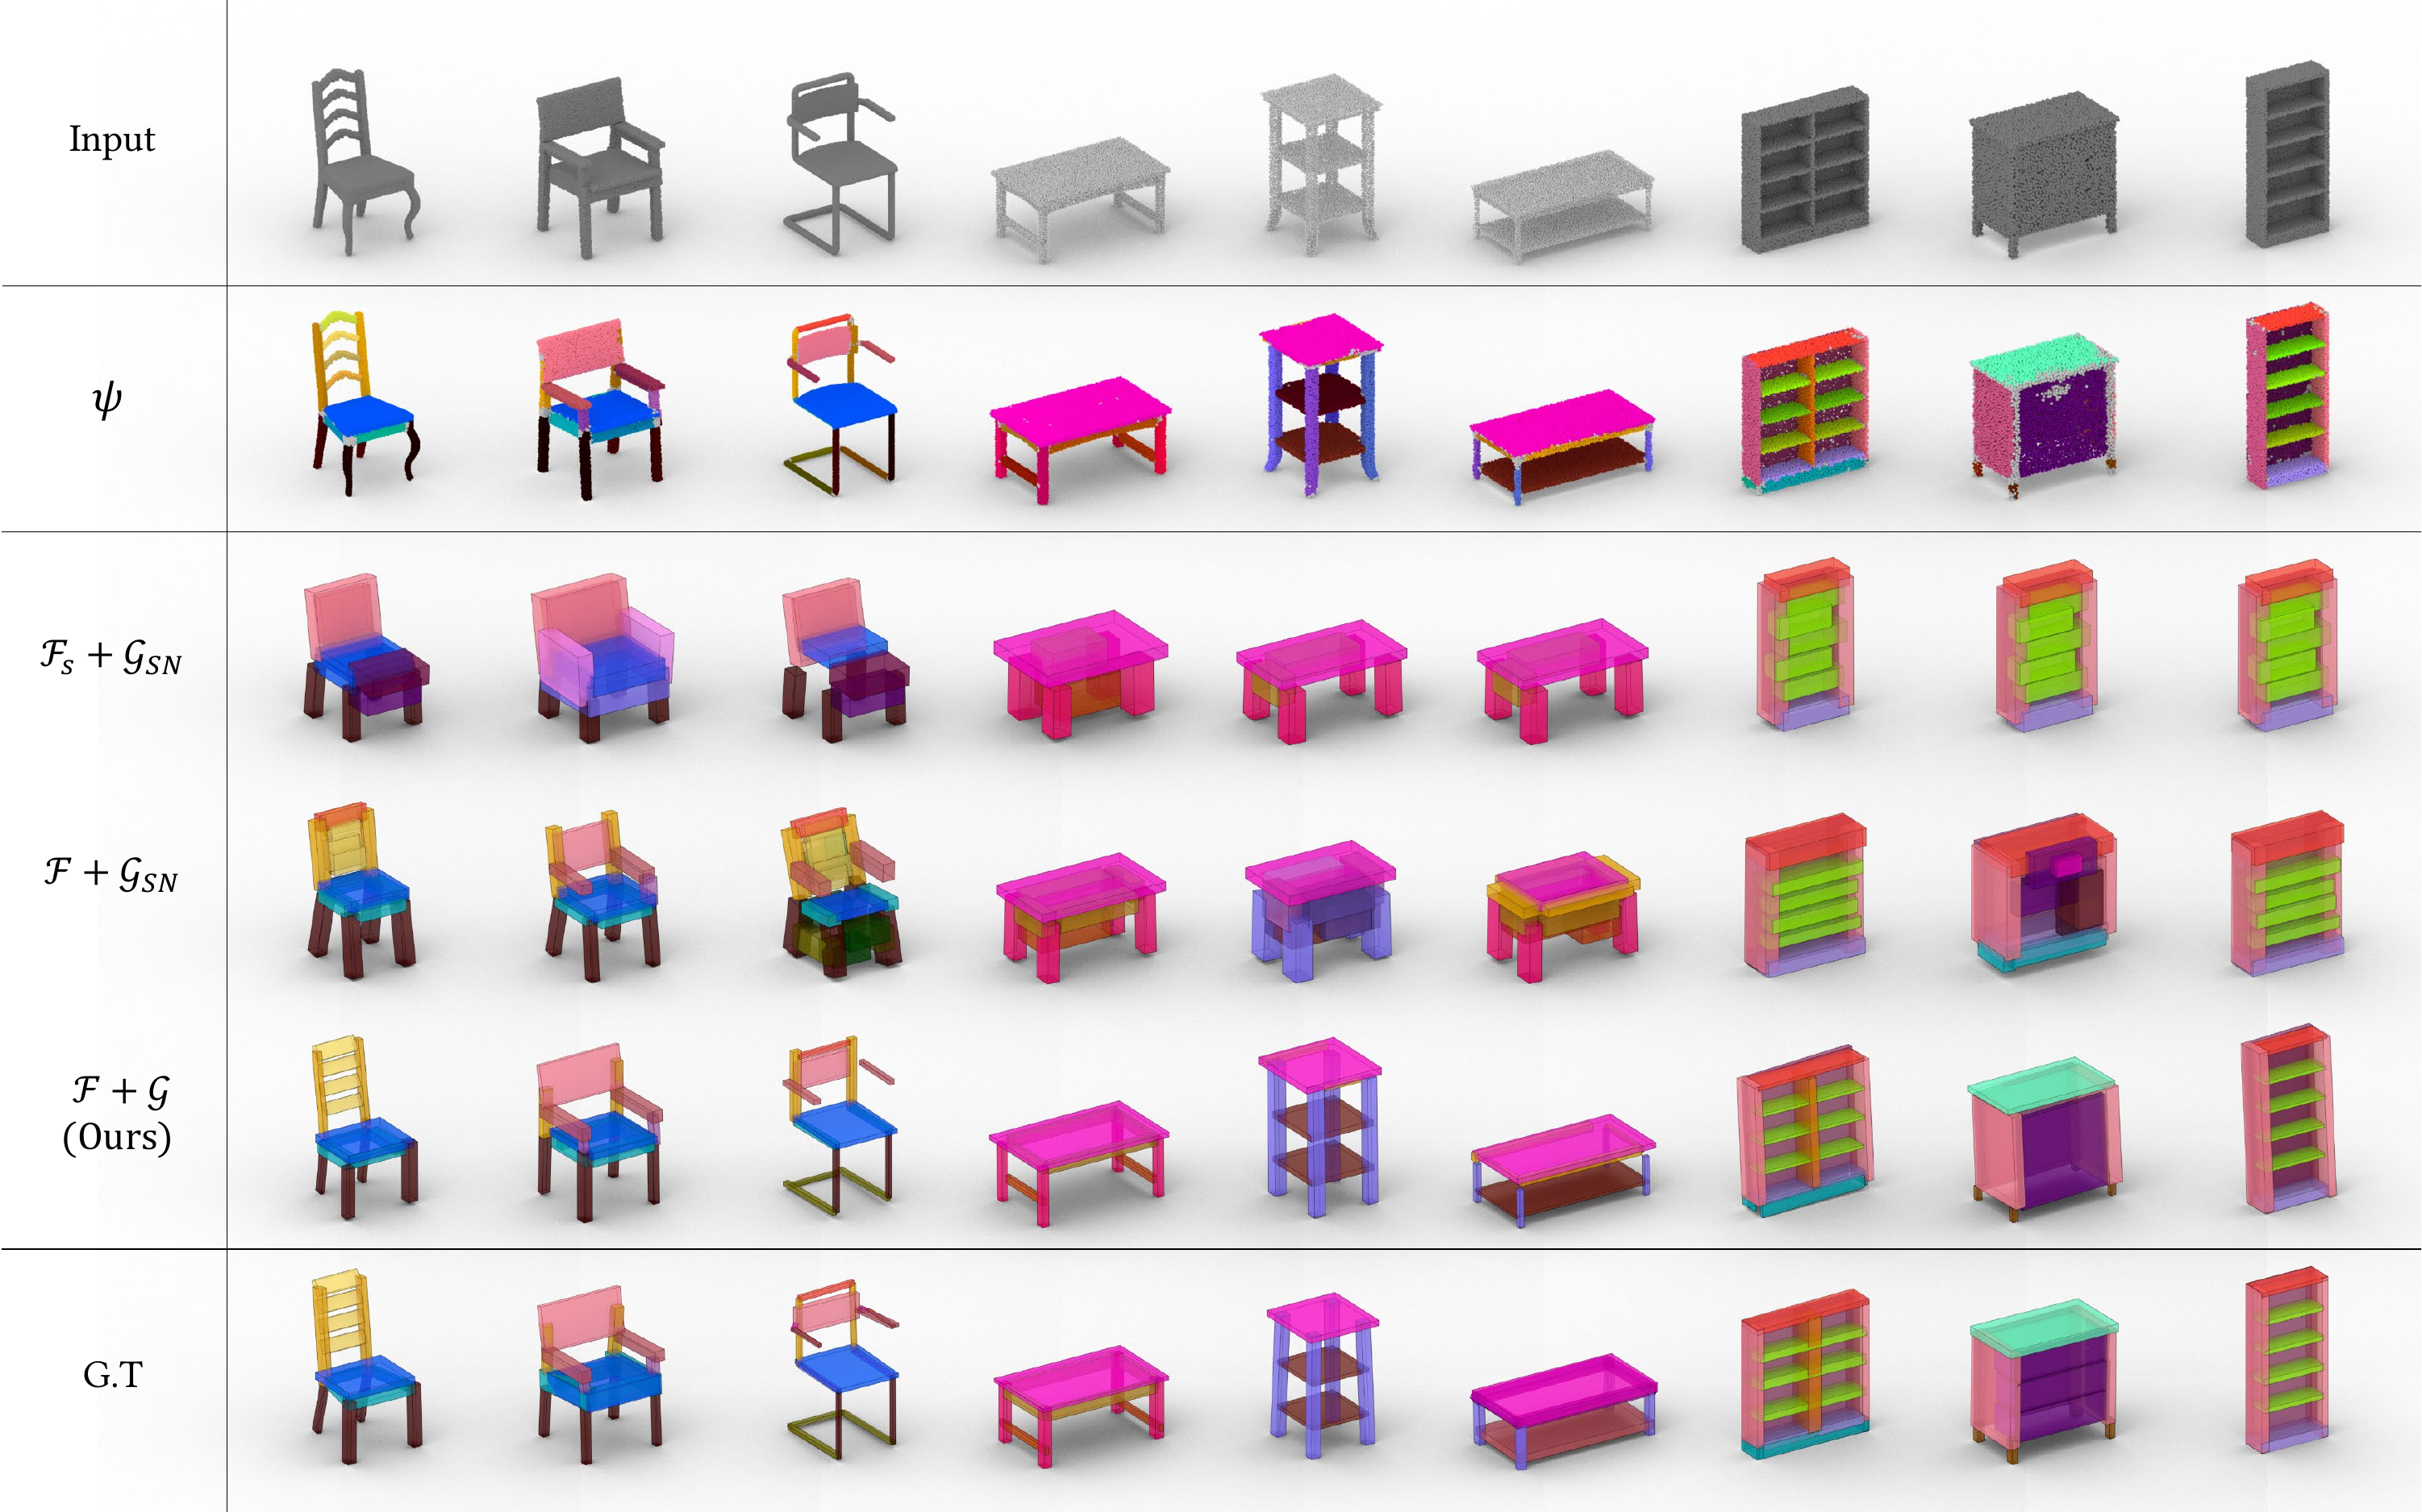}
    \caption{\textbf{Qualitative Comparison on Structure Inference.} The top row describes the input 3D shape and the bottom row describes ground-truth. In the second row, the part segmentation outputs from $\psi$ are shown. The results from baselines are not accurate and only output a few set of part structure (See storage furniture case). Compared to others, ours achieves the most accurate part structures by fully exploiting segmentation and hierarchy priors. }
    \label{fig:results}
\end{figure*}

\subsubsection{Quantitative Results.}
We demonstrate our quantitative evaluation results in Table~\ref{tab:comparison}. 
Obviously, ours outperforms the naive encoder-decoder baselines (first and fifth rows) in two metrics, leaving significant margins for both.
The numbers in the first row describes the prediction results without prior knowledge our method uses, i.e. hierarchy and part segmentation priors.
We find utilizing those priors extremely helpful, while the one without them fails obviously. 
By comparing it with ours (eighth row), we can see the significant margin by 30.94\% in part prediction accuracy and 0.2713 in edge prediction error, 
Empirically, we observe that naively encoding raw geometry cannot contain any useful information so that the decoder outputs only a few set of structure outputs. % \Jeonghyun{Figure for this?}

The other baseline without skip connection (fifth row) do not achieve good results neither, only with the small improvement.
Since this one takes the latent code aggregated in hierarchy, the edge prediction error reduced and the structure prediction accuracy slightly increased.
However, the overall performance still remains unacceptable and the decoder fails to cover more diverse sets of structure in the shape collections. % \Jeonghyun{Figure for this?}  YES

Compared to other baselines, we can see the significance of our method (eighth row) set up on association between part segmentation outputs and constructed structure hierarchy.
Another remarkable finding in our experiments comes from the improvement induced by an \emph{interplay} between part segmentation and structure prediction.
We observe the refined structure prediction based on the refined segmentation from merge prediction $\mathcal{M}$ outperforms the initial prediction results by 1.5\% in average. 
This result supports the rationale for our motivation, the interplay between segmentation and structure to build a synergy between them, as both tasks are improved by supporting each other.

\begin{figure*}
    \centering
    \includegraphics[width=\textwidth]{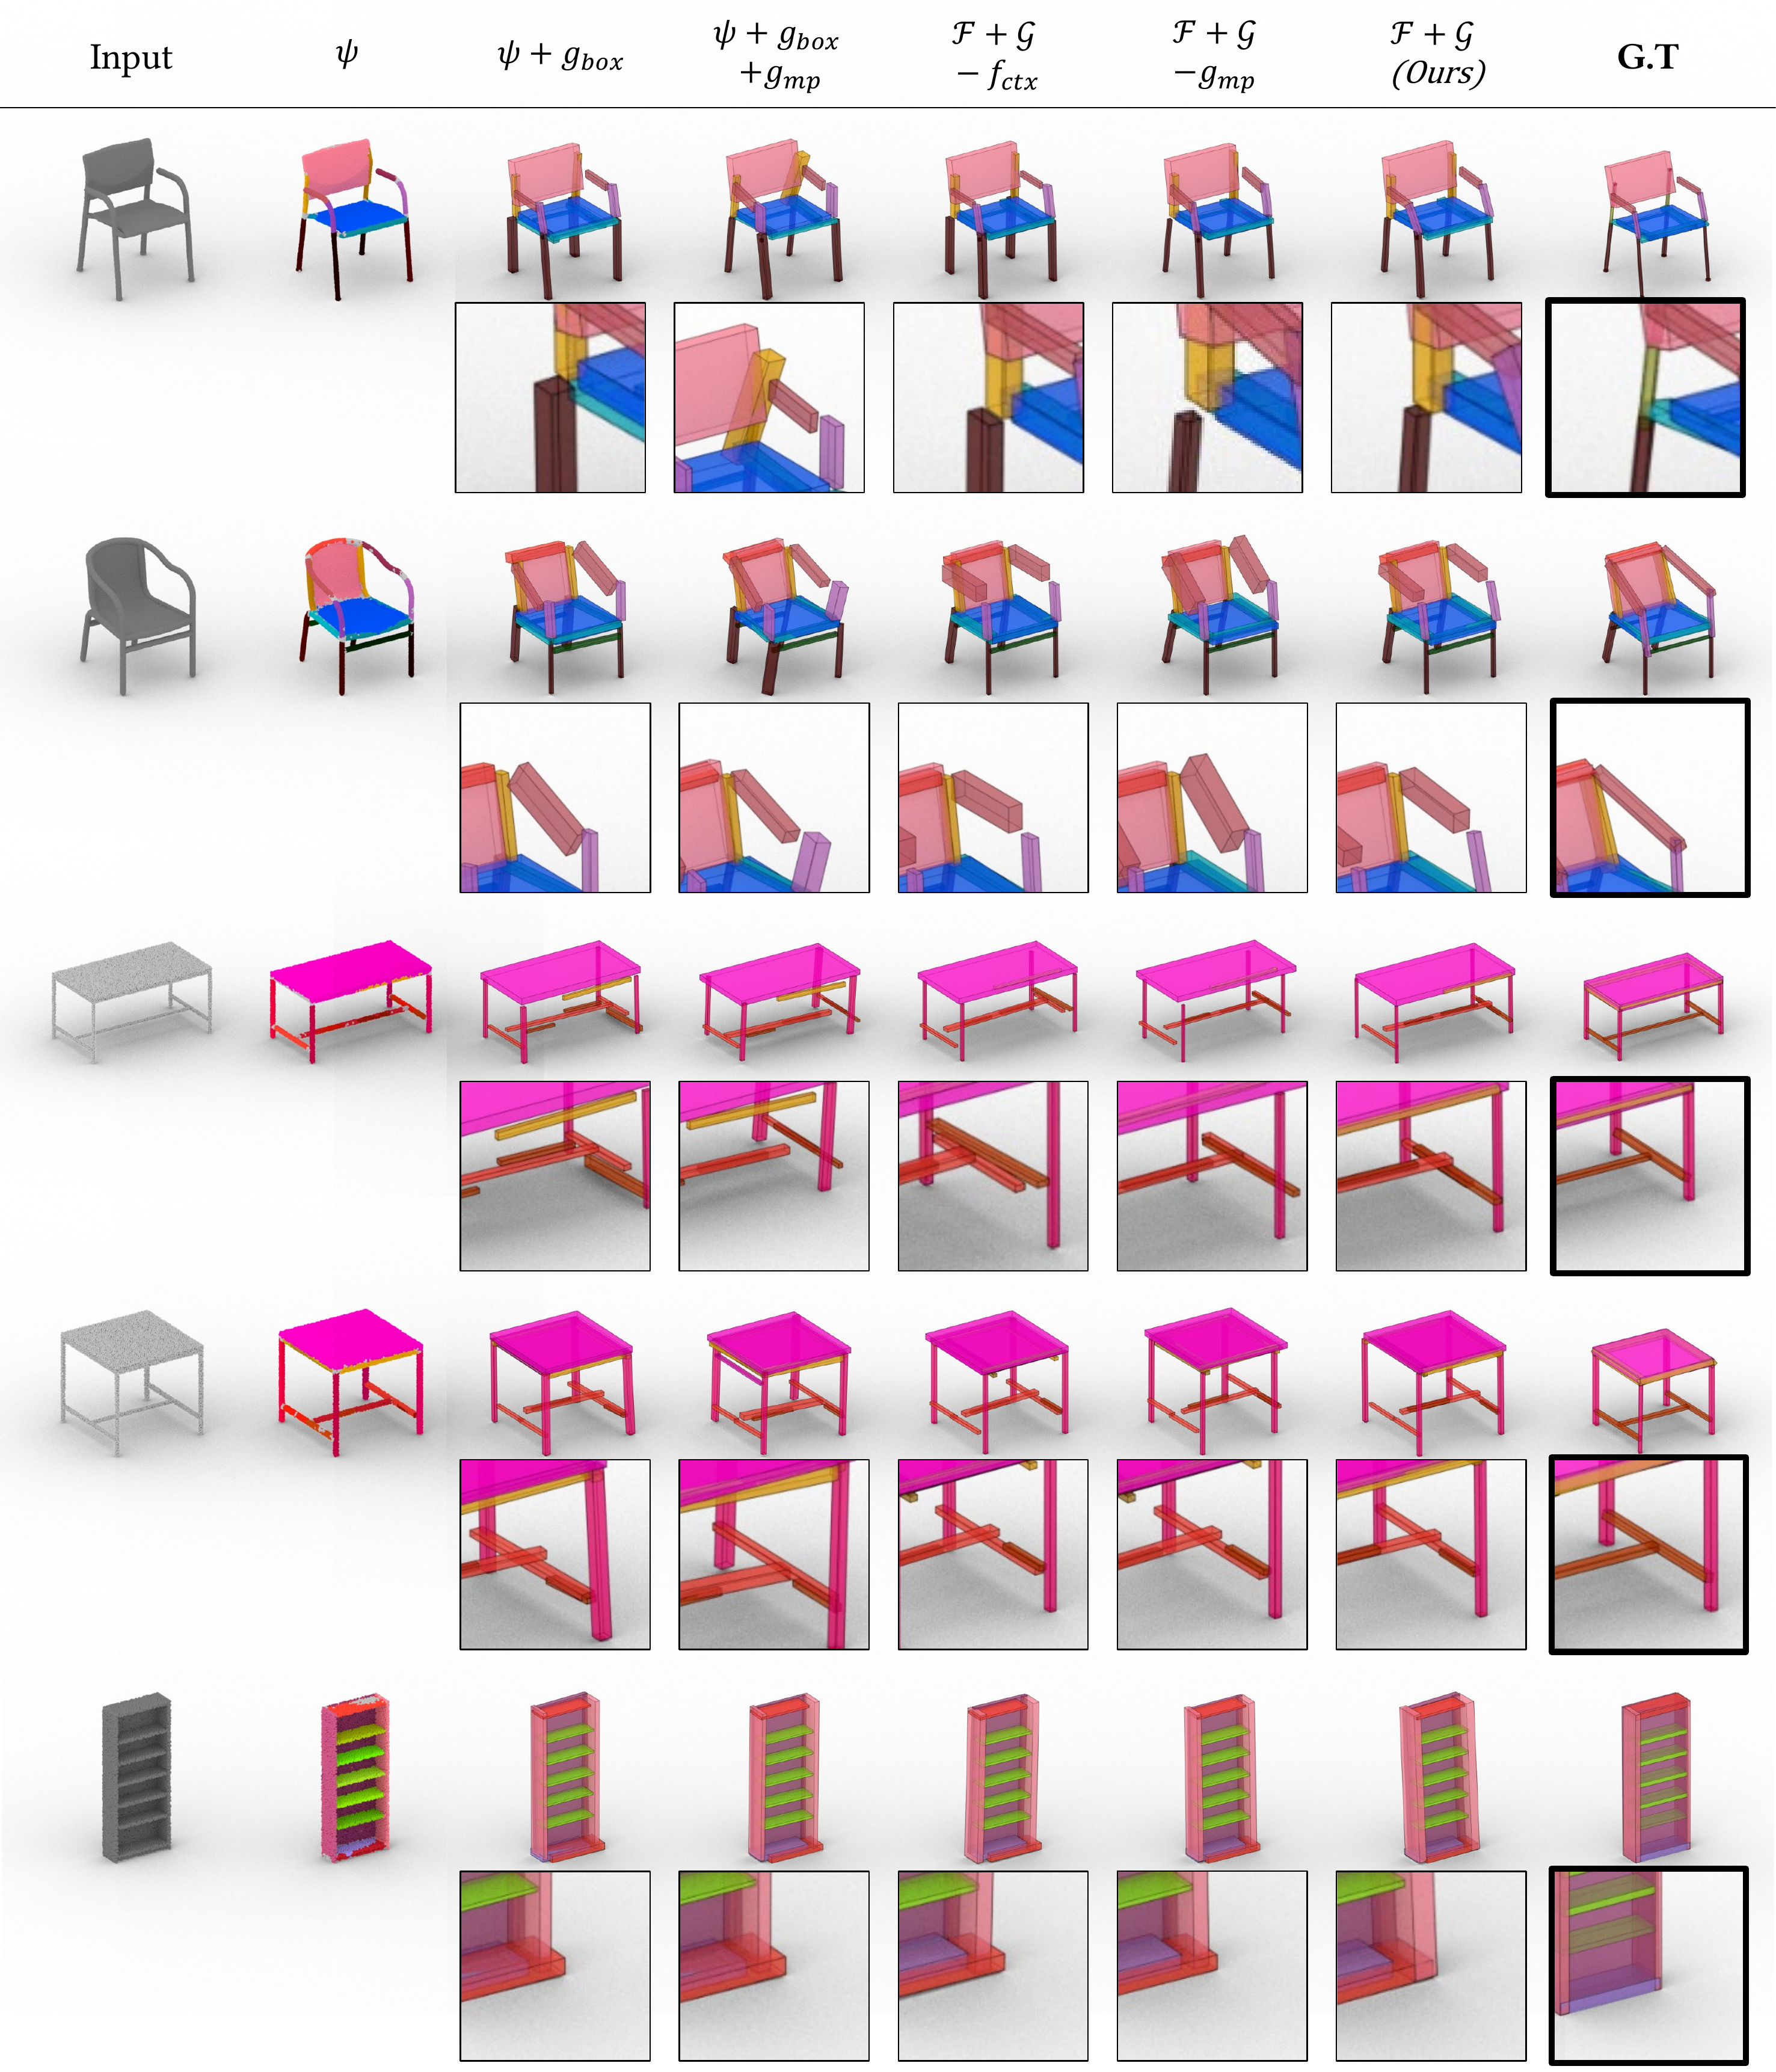}
    \caption{\textbf{The illustration of Ablation Study on Hierarchical Message Passing.} The zoom-in images for each case describe how this improvement enhances the structure output more clearly. As our key components for hierarchical message passing applied, the overall arrangement of part structure improves.}
    \label{fig:ablation}
\end{figure*}

\subsubsection{Qualitative Results.}
We illustrate the qualitative results for comparison in Figure~\ref{fig:results}. 
For the first, the second row and the bottom rows, we depict the raw input geometry, the part segmentation output from $\psi$, and the target structure, respectively. 
Clearly, our method predicts the most plausible structures resembling the target, compared to other baselines.

As illustrated, other baselines almost deliver inaccurate appearance even from given input shape and less realistic structure.
Even in the case of an approximate structure predicted, they fail to recover the precise part geometry of small and thin parts.
The second baseline (fourth row), in particular, also fails to transfer the information of part regions extracted to decoding step, although the clear correspondence exists.
We observe that this naive encoder-decoder method completely miss not only the accurate structure prediction performance, but also the diversity of output structure.
The output structures from the baselines have similar appearance, given apparently different input shapes.

On the other hand, our method produces desirable outputs for all categories even for the cases of complex input geometry, by fully utilizing part segmentation outputs and the association between part regions and part structure.
% \Jeonghyun{Description for each category?}

\subsubsection{Ablation Study}\label{Sec:6.4.3}
To demonstrate the effectiveness of the key components in our proposed our hierarchical message passing $g_h$, we perform sets of ablation studies. 

\textit{Baselines.}
Here, we built an another type of baseline, which directly decodes the bounding box from extracted part instances. 
Based on our backbone $\psi$ and the part feature encoder $f_{part}$, the box decoder baseline parses the input shape into leaf part instances, encodes part features, and directly predicts bounding box parameters~$\{\theta_l\}_{l\in L}$. 
Here, we prepare three kinds of box decoder baselines ($2^{nd}-4^{th}$ rows in Table~\ref{tab:comparison}) directly consuming the output from backbone $\psi$: a PCA-based bounding box estimator, a box decoder $g_{box}$, and the box decoder with message passing network $g_{mp}$.
Since these box encoders except the last one do not predict and learn any part relations, the edge prediction error is not measured.
Note that the last one uses the reduced version of our part-relation learning where the relationships are learned across all the leaf instances, which makes the edge prediction a lot difficult.
Then, we show how the level of feature updates in the local part-relation learning and global context learning affects the performance of structure inference for each.
To this end, we built baselines by subtracting each component of $g_h$ from our framework~$\mathcal{F}+\mathcal{G}$, represented as the one without local part message passing $g_{mp}$ and global context encoding $f_{ctx}$. % ($6^{th}-7^{th}$ rows in Table~\ref{tab:comparison}).

\textit{Results.}
We observe that our method based on hierarchical message passing beats the other baselines quantitatively in Table~\ref{tab:comparison}.
For the baselines with different level of structural context, the mean part prediction accuracy also increases.
We find that learning global context even helps to improve the local part relation classification in average, which supports the necessity of our hierarchical message passing.
While the box decoder with leaf parts message passing shows compatible part prediction accuracy to ours, it extremely suffers to predict the precise part-relationships with the highest edge prediction error.
We illustrate how this negatively affects to predict the globally consistent structure in Fig.~\ref{fig:ablation}.

As we gradually added the key component of our method, the leaf parts are coherently arranged by learning hierarchical relationships in the structure (from left to right). 
Despite of the precise quality of the part segmentation output, the compared baselines fail to capture co-relations between parts across the structure.
For the box decoder baselines in the third and the fourth column, some parts pop out and degrade the overall assembly quality.
Even with part relation learning, the \emph{symmetry} between nodes is easily corrupted~(see the \emph{chair} cases).
The cases of shapes with cluttered set of parts~(see the \emph{table} cases) get much severe where the \emph{adjacency} between parts is broken resulting in the scattered output.

For the baselines subtracting the key component of hierarchical message passing, we also found that incorporating all the context information achieves the most plausible results. 
Although the edge prediction quality seems to have relatively small margin in numbers (Table.~\ref{tab:comparison}), we observe there is a more clear improvement in visuals.
While the symmetry between parts are preserved better than the box decoder baselines, we observe that missing one of the structural context still yield flawed prediction with broken adjacency.
As each context is added, we observe the part structure accomplish \emph{globally-aligned} arrangement even with the cluttered set of parts.
For example, in the first chair case, the adjacency and alignment between a leg (brown box) and a vertical frame (yellow box) become consistent.

\subsection{Structure-to-Segmentation Refinement}\label{Sec:refinement results}
Next, we present the experimental results for our structure-to-segmentation refinement, the \emph{reverse} process on top of the structure inference.
In the quantitative and qualitative evaluations, we discuss how the proposed method refines the quality of the given part segmentation output.
Since we do not train any additional part segmentation network in our framework, we will focus on the \emph{improvement} on the segmentation quality from our backbone $\psi$.
For quantitative measurement, we use a class-wise \emph{mean Average Precision (mAP)} with IoU threshold 0.5, which is the most widely used metric for this task.
From the results, we observe our method marginally improves the initial segmentation, predicting the accurate merge operation utilizing the multiple structure-aware features.

\subsubsection{Baselines}
We compared our method to the other state-of-the-art part segmentation method, covering SGPN~\cite{wang2018sgpn}, PartNet~\cite{mo2019partnet}, Probabilistic Embedding~\cite{zhang2021point}, and PointGroup~\cite{jiang2020pointgroup} on PartNet dataset.
While the original evaluation on PartNet benchmark calculates all the level of part annotation, we only represent the results for the most complex level since the hierarchy annotation from StructureNet is based on that. 
To show the necessity of our proposed method using structure-driven refinement approach, we compare ours to another simple baseline that predicts merge operation directly from the output from part segmentation.
We use the part geometry based candidate feature $\textbf{c}_i$ only (see Section~\ref{4.3}), and the merge candidates are detected from a PCA-based box decoder, analogous to the one from our ablation study (second row in Table~\ref{tab:comparison}).

\subsubsection{Results}
We demonstrate the result of quantitative evaluation in Table~\ref{tab:refine}.
Before our merge prediction, we observe that PointGroup itself achieves the state-of-the-art performance on part instance segmentation overall.
We observe that this quality can be much enhanced after structure-driven merge prediction (bottom row), showing the improved segmentation accuracy by 0.6\% in average.
However, for our compared baseline, we observe that the accuracy rather decreases in average, where the merge prediction is not aware of the structure information and depends on the part segmentation results only.
Even for the improved categories, the margins are up to 0.1\%, which is much smaller than ours.
For chair category, the number seems not improved that much since the most of the chair part segments are relatively small to make bigger improvement even though with the correct merge prediction.
On the other hand, the other categories have the bigger improvement where most of the merge cases occur in the bigger part regions. 
We provide the visualization of this refinement process for clearance in Fig.~\ref{fig:refine}.
As discussed, we also observe that this refined segmentation can again be used to improve the predicted structure, closing the interplay, leaving a big margin by 1.5\% in part prediction accuracy (Table~\ref{tab:comparison}).

Fig.~\ref{fig:refine} illustrates how the merge operation gives us the refined part segmentation and part structure.
Given an initial segmentation output and the prediction structure from it, we first predicts merge operation by $\mathcal{M}$ for the candidate nodes detected by the conflict of the part boxes.
After merging the candidate part node to its target node, we refine the part segmentation and also the predicted part structure as well. %and the corresponding part segments.
For the chair case in the top, two vertical boxes at the right chair arm region (the orange and purple colored ones) collide to each other, making an overlap. 
For the storage furniture case in the bottom, we can easily see the collision occur on the top of the shape (the red and cyan colored ones). 
Based on this conflict information, we predict merge operation for these parts and refine the initial part segmentation fully utilizing the set of structure-aware features (see Section~\ref{4.3}).
From the visuals, we observe the accurate merge prediction gives us much realistic and clear outputs, both the part segmentation and the part structure.
We provide more examples in Fig.~\ref{fig:refine_all}.

\begin{table}[]
\caption{Quantitative Evaluation on Structure-to-Segmentation Refinement. The numbers are calculated by mean average precision (mAP) for each part semantic in the shape category. Compared to PCA-based baseline which rather decreases the performance, ours with structure-aware features has shown clear advantage of proposed method. }
\begin{tabular}{lcccc}
\hline
                  & \multicolumn{1}{l}{Avg} & \multicolumn{1}{l}{Chair} & \multicolumn{1}{l}{Stora.} & \multicolumn{1}{l}{Table} \\ \hline
SGPN~\cite{wang2018sgpn}                & 18.5                    & 19.4                      & 21.5                       & 14.6                      \\
PartNet~\cite{mo2019partnet}            & 26.8                    & 29.0                      & 27.5                       & 23.9                      \\
PE~\cite{zhang2021point}                & 31.5                    & 34.7                      & \textbf{34.2}                       & 25.5                      \\
PointGroup~\cite{jiang2020pointgroup}   & 32.7                    & 40.7                      & 26.8                       & 30.7                      \\ \hline
PointGroup + PCA-box                    & 32.3                    & 40.7                      & 26.9                       & 29.4                      \\
PointGroup + \ShortName{} (Ours)               & \textbf{33.3}                    & \textbf{40.8}                      & 27.5                       & \textbf{31.6}                \\ \hline
\label{tab:refine}
\end{tabular}
\end{table}

\begin{figure}[]
    \centering
    \includegraphics[width=0.48\textwidth]{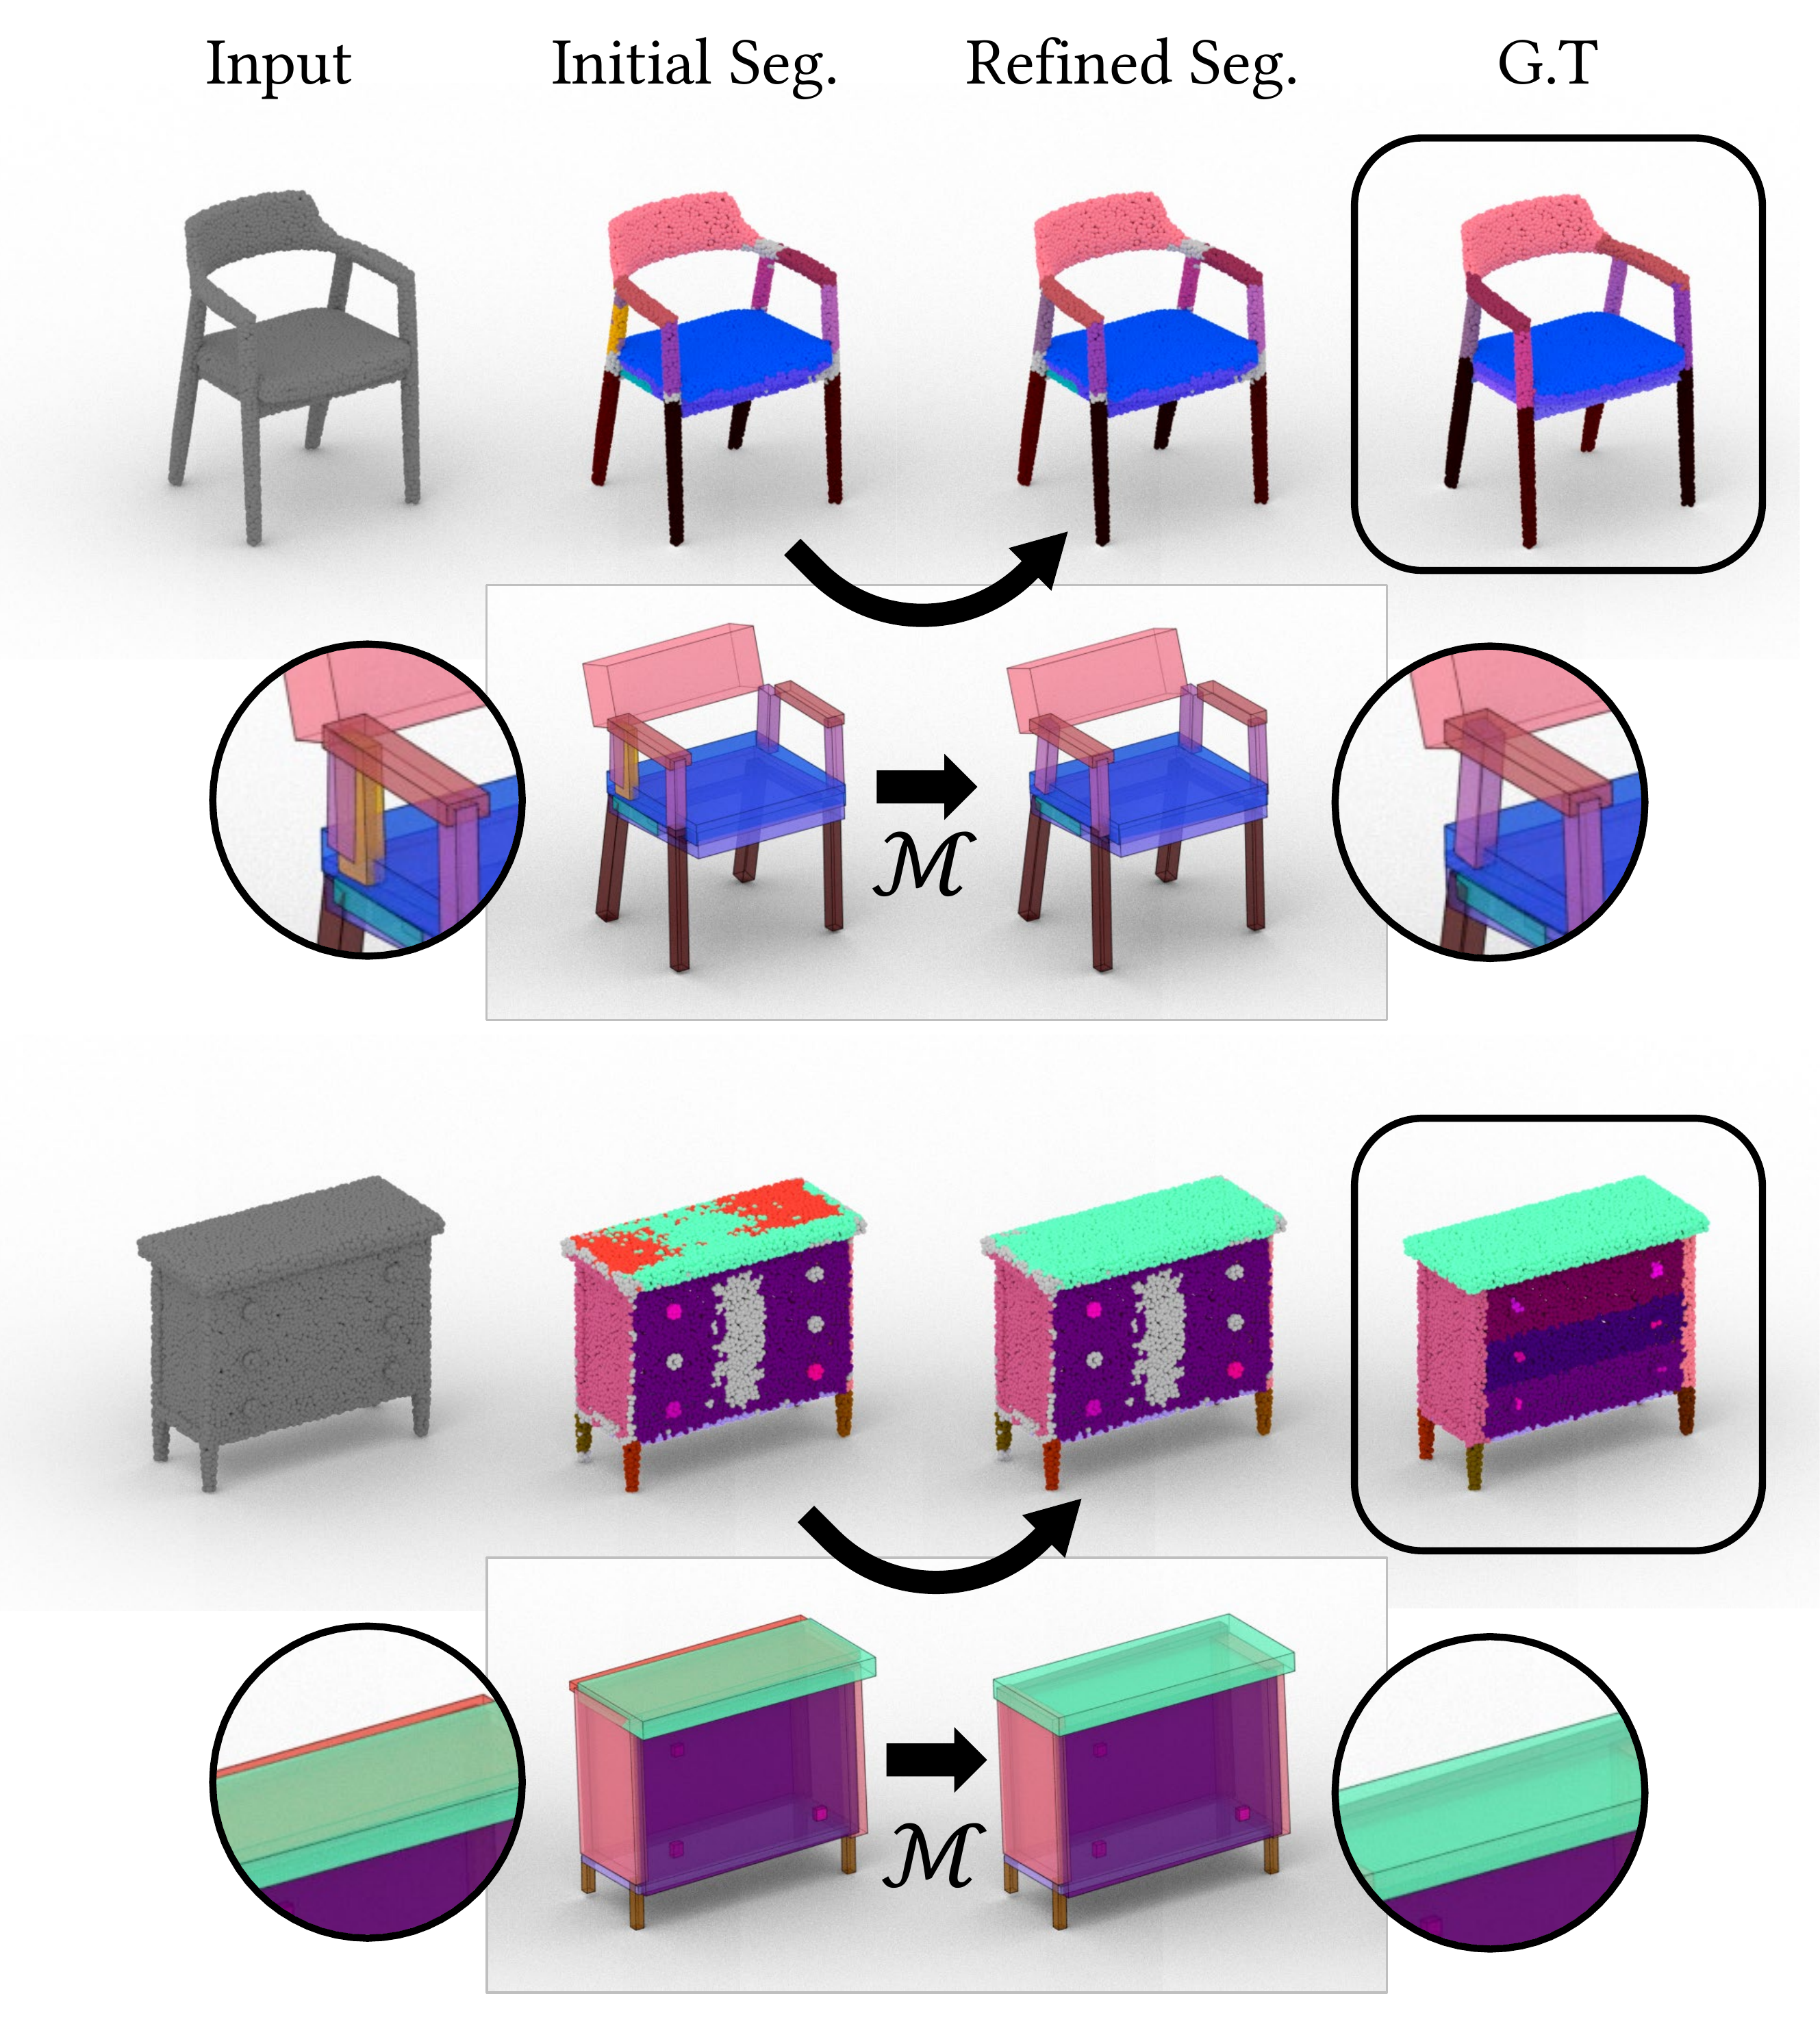}
    \caption{\textbf{Structure-to-Segmentation Refinement.} Utilizing structural information from forward structure inference step, we improve the initial part segmentation using refinement network $\mathcal{M}$. The circle describes a closer look for the region of conflict in the predicted part structure. After merge prediction, we can get refined segmentation removing noisy regions.}
    \label{fig:refine}
\end{figure}

\begin{figure*}
    \centering
    \includegraphics[width=0.95\textwidth]{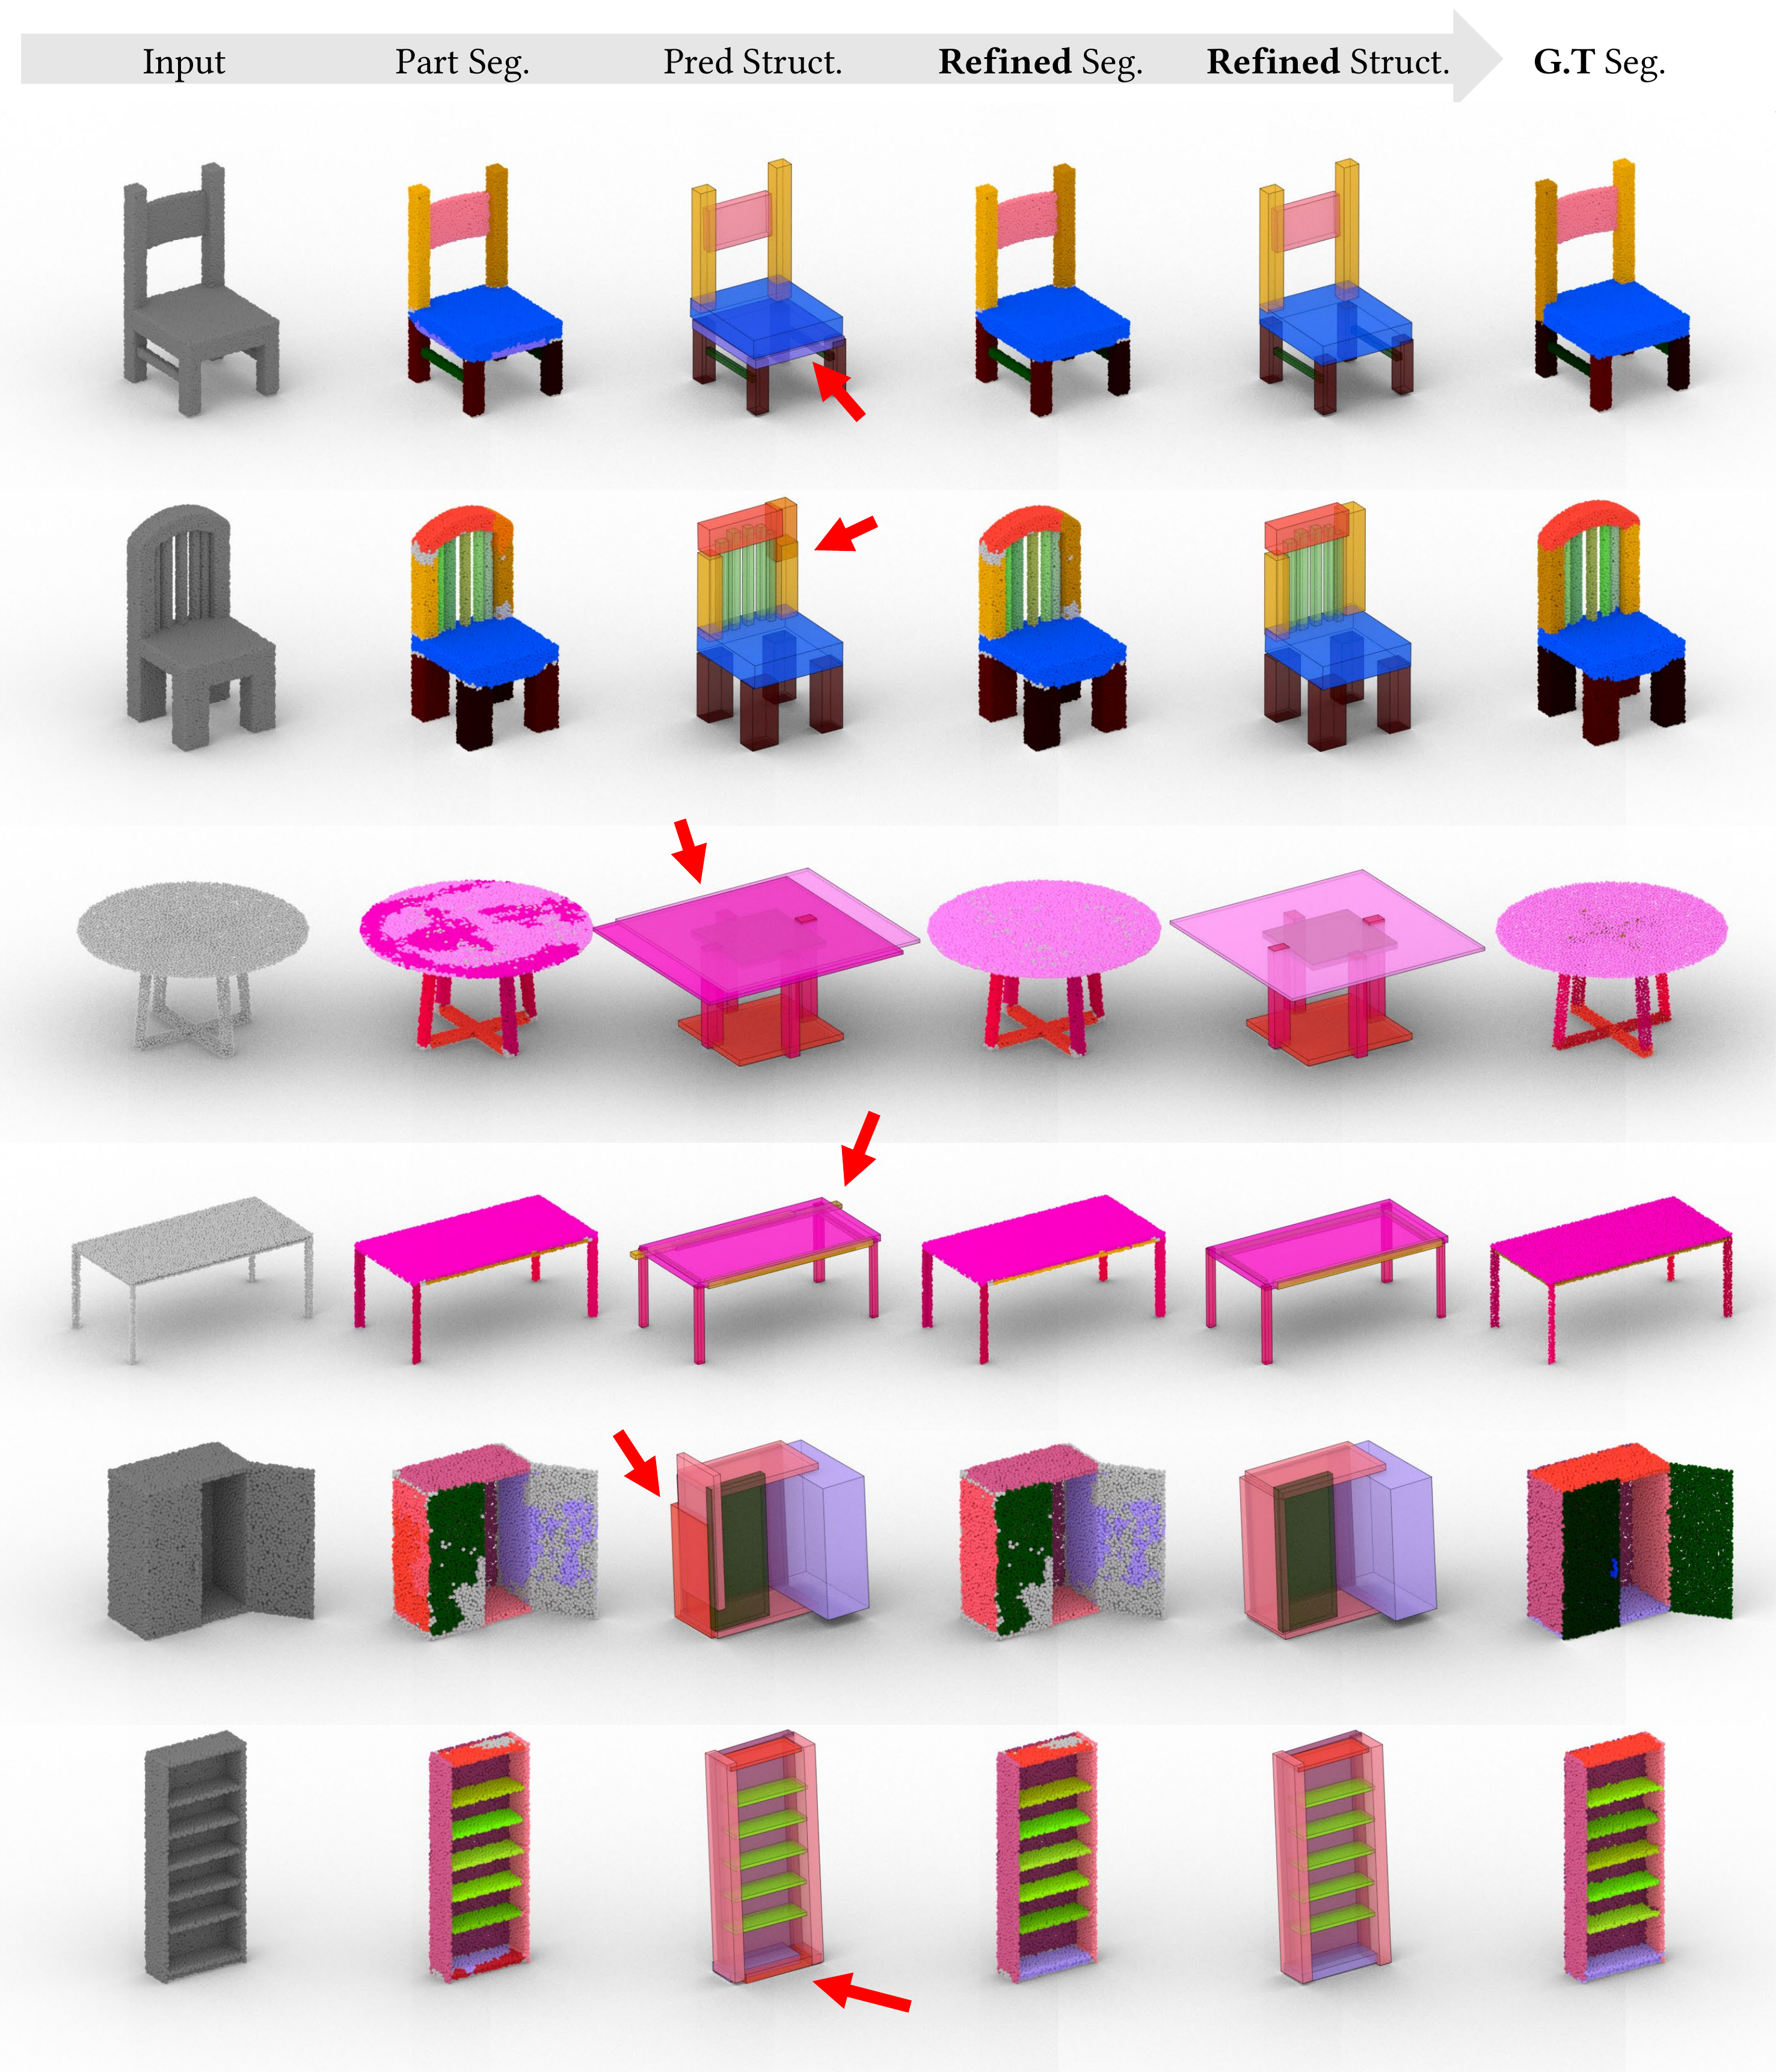}
    \caption{\textbf{More Results of Structure-to-Segmentation Refinement.} The ground-truth part segmentation is at right-most column. We point the region of conflict using red arrow. Our refinement successfully improve the quality of segmentation and structure both, covering diverse merge cases for all categories.}
    \label{fig:refine_all}
\end{figure*}

\begin{figure*}
    \centering
    \includegraphics[width=0.95\textwidth]{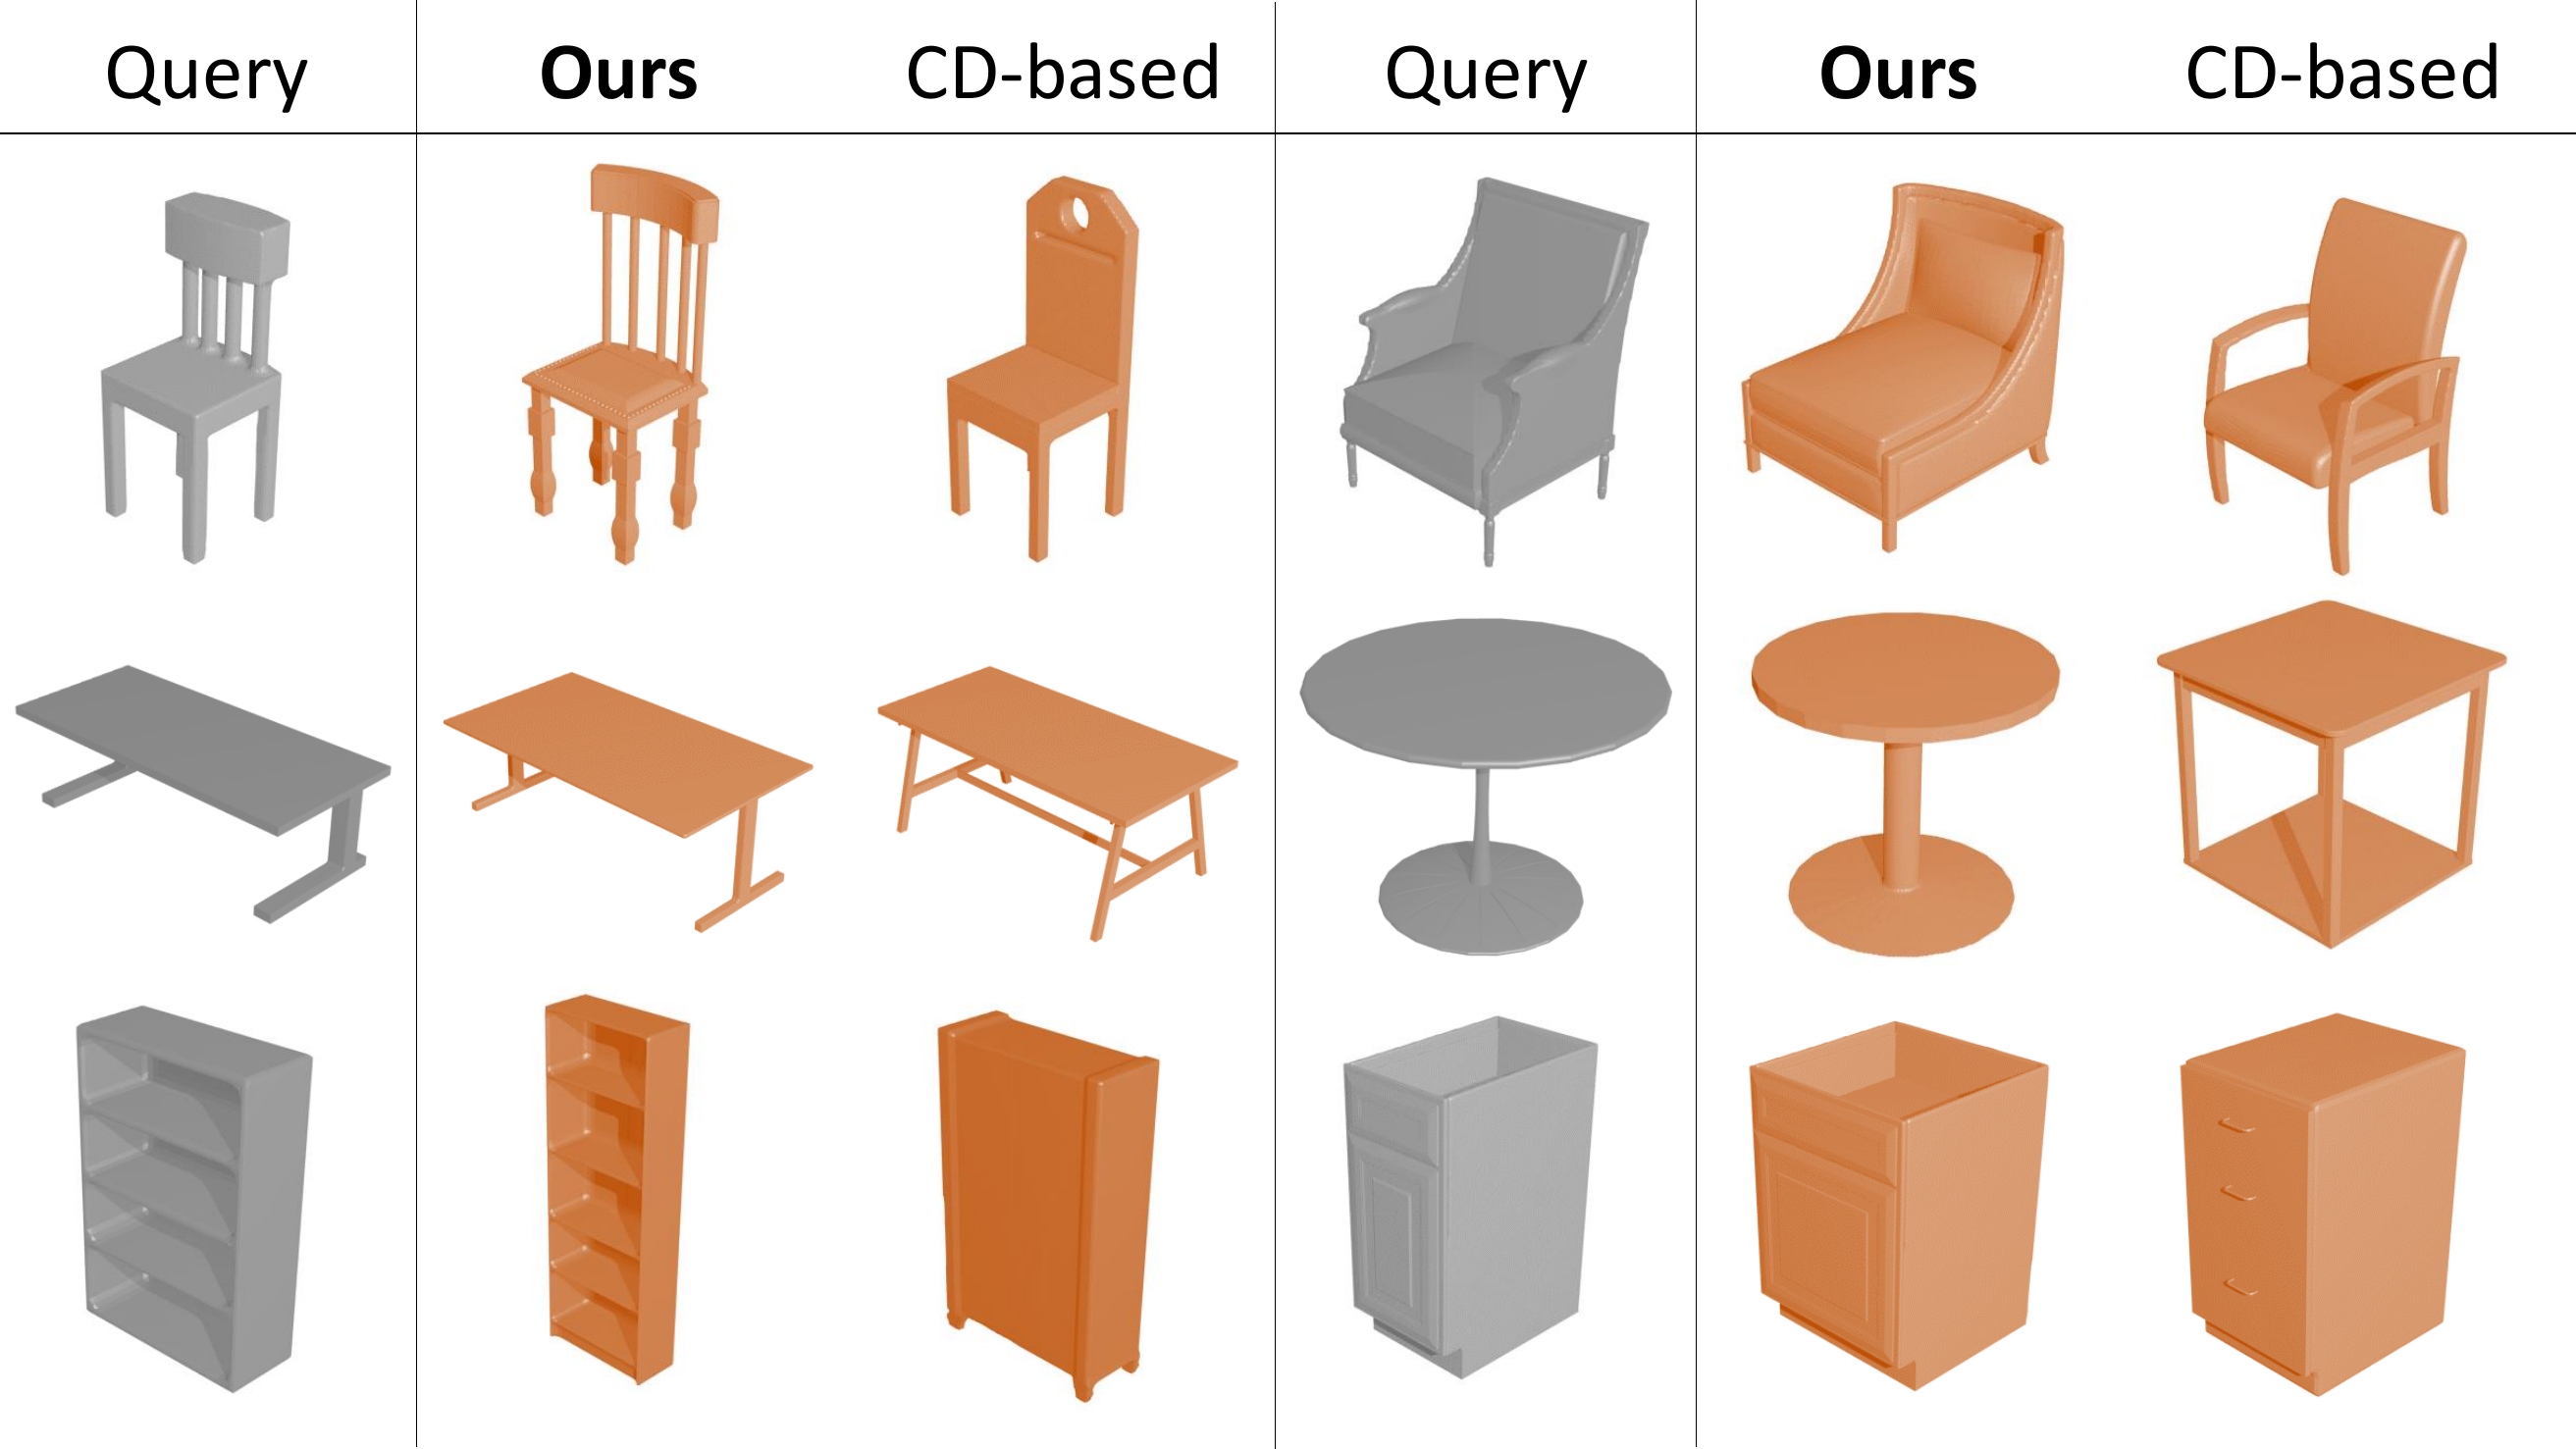}
    \caption{\textbf{Structure-aware vs. CD-based Shape Retrieval.} We showcase a Top-1 retrieval results to compare two approaches.}
    \label{fig:retrieval}
\end{figure*}

\subsection{Structure-aware Shape Retrieval}
The shape retrieval, which is to search the most resemble shape in the database given a query shape, has been one of the most practical application upon the shape difference measurement.
Currently, there has been a typical and dominant approach to comparing two shapes by measuring a \emph{fitting distance}, which is usually computed by chamfer-distance (CD). 
This yields a perceptional failure cases where we seek to find the similar shape in perspective of the semantic and structure, rather than the CD-based fitting distance.
However, with the closest fitting distance, it is not guaranteed that the retrieved shape shares similar structural information with query shape (Figure~\ref{fig:retrieval}). 
This limitation of CD-based shape retrieval has not been considered, even for the the state-of-the-art methods~\cite{avetisyan2019scan2cad, dahnert2019joint, uy2020deformation, uy2021joint}.

To tackle this, we propose a \emph{structure-aware} shape retrieval as an application based on our proposed framework.
Given query 3D shape with raw geometry, we measure a \emph{structure difference}, reflecting the similarity of semantics between the query shape and shapes in the shape collection.
Ours can achieve this through structure inference beyond depending on the raw 3D geometry data only. 
To measure the structure difference, we compute the number of matched parts for semantic label classification accuracy based on the established correspondence $\textbf{M}$ in our training (See Sec~\ref{4.2}).
Thus, we compare the query shape to the shapes from database to find a shape that shares the largest number of the same semantic parts in the hierarchy.
On the other hand, the baseline adapts the squared version of chamfer distance~\cite{achlioptas2018learning} to calculate fitting error using the points sampled from surfaces of the shape. 
In the evaluation, we prepares all shapes in the test set from PartNet.
We take these shapes as queries and retrieve shapes from the same database except for the query shape.

\subsubsection{Qualitative Results}
We showcase the results of top-1 shape retrieval comparing our structure-aware retrieval with the chamfer distance baseline in Fig.~\ref{fig:retrieval}.
For all three categories, ours shows that it address the failure cases occurring in CD-based approach.
We observe CD-based shape retrieval often fails to reflect the structural similarity for semantic parts even with the minimum fitting error in geometry.
For examples, in the first case of the storage furniture category, fitting distance cannot detect the existence of \emph{legs}.
On the other hand, ours can find shapes with the similar semantic parts given query shape using the predicted structure, beyond the geometry measurement.
For each case in the visual, we find the output from our method does not yield the smallest fitting distance, while the retrieved shapes are more similar \emph{semantic} parts, e.g. the first case of chair category and the second case of the storage furniture. 
However, We observe that this is not achievable using CD-based approach where.
% We observe that this is not achievable using CD-based approach.

\subsection{Limitations}
We observe that our segmentation refinement method suffers from the imperfect supervision given by the noisy annotations.
For similar shapes, there are noisy annotations that make our network hard to predict the correct merge operation.
In Figure \ref{fig:failure}, we illustrate these failure cases caused by the noisy annotations.
For example, given almost the same shapes in Chair category, the leg part (dark brown) is hard to be distinguished from the foot part (orange) even for the annotators.
When these confusing labels are found in the part boundaries, the network cannot clearly describe which part is falsely segmented and also examine the direction of the merge process correctly.
Unfortunately, we found these failure cases also happen across the other categories. 
Since our framework solves a supervised problem for the part segmentation, these noisy annotations largely restrain the improvement on the structure-to-segmentation refinement task and the further refinement on the part structures. 

\begin{figure}[t]
\begin{center}
\includegraphics[width=\linewidth]{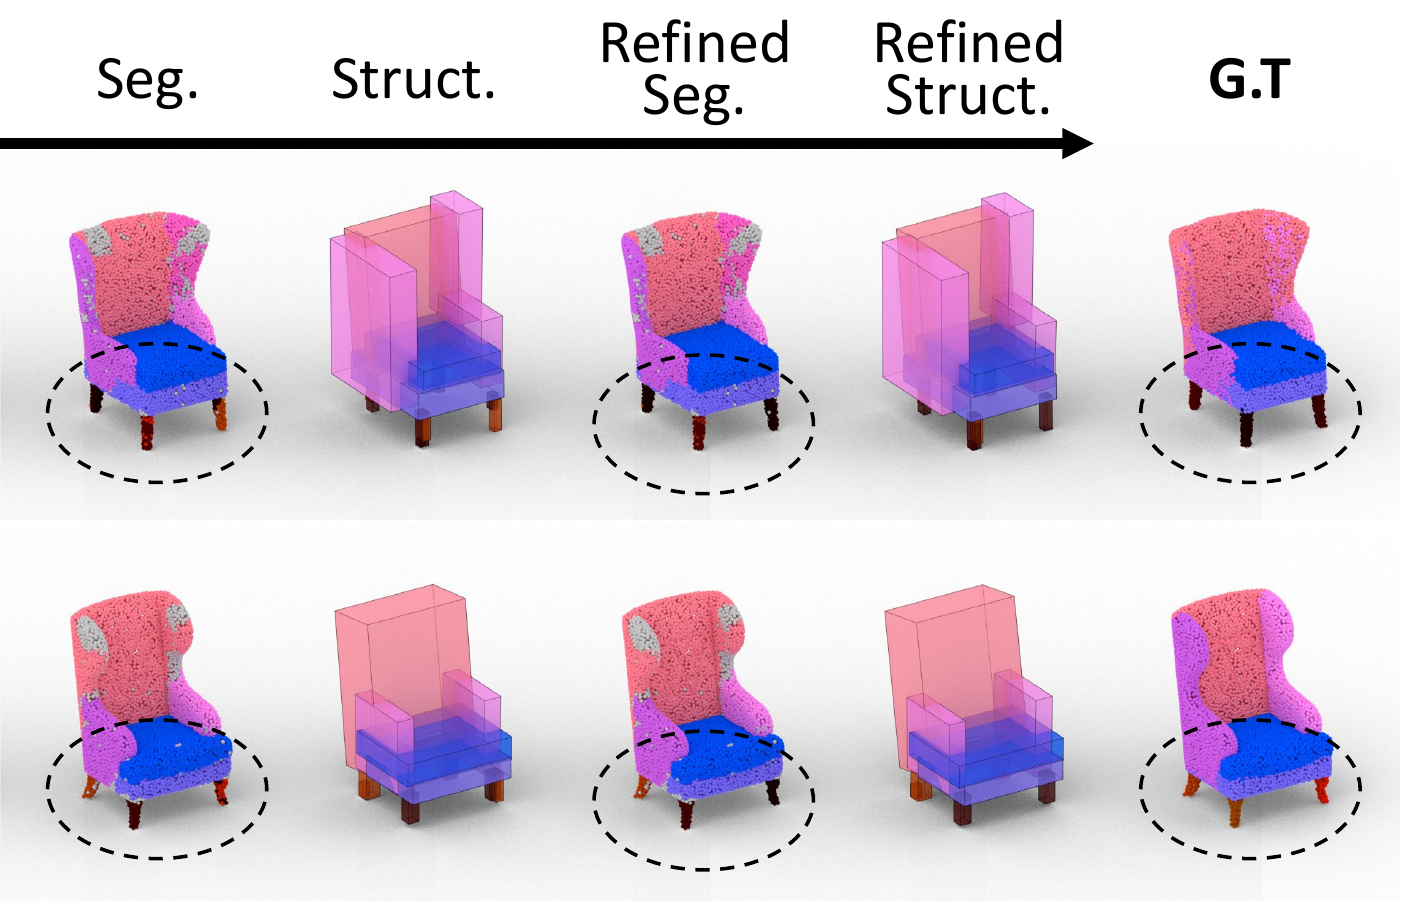}
\end{center}
   \caption{\textbf{Failure Cases}. Both shapes in two rows share the same Chair category. However, noisy labeling on the same region by human annotators, the orange color for \emph{foot} part and the dark brown color for \emph{leg} part, confuses the network to predict correct merge operations and yields false outputs.}
\label{fig:failure}
\end{figure}

% \section{Results}
% In this section, we demonstrate how our proposed pipeline accurately decomposes a structure from raw input geometry through quantitative and qualitative evaluations. 
% Our final baseline has shown its significance to reconstruct structure geometry and predict part-relations, incorporating both local and global structural contexts hierarchically.
% The experimental results show our method adapting multi-level structural context learning outperforms other baselines.
